# Supplementary material for: Computing properties of thermodynamic binding networks: An integer programming approach
Source: arXiv:2011.10677 source file (2021-05-12)
Supplement: Supplementary file 1 [file appendix.tex]

%old sections: to be removed, incorporated, or placed in appendix
\todoi{-----------------------------------------\\
Sections below this will be removed, incorporated, or placed in the appendix}
\section{StableGen Reminders}

In this section I summarize the relevant sections of the paper by Breik, Thachuk, Heule, and Soloveichik \cite{tbn-sat} which inform the current implementation of the StableGen software (\url{http://stablegen.net}).

In this version of this document, I assume that the reader is familiar with the definition of Thermodynamic Binding Networks (TBNs) as presented in \cite{tbn, tbn-sat, ktbn}; however there will be some modifications to the model (in particular, to allow for multisets and for infinite quantities of monomers) which will be described more fully in the complete version of this document.
\todom{DH: Formalize the concept of $\infty\cdot$TBNs}

In particular, the original work describes the following decision problem (Definition 1 in \cite{tbn-sat}):

\begin{definition}
($\mathcal{T}$, $k$) is in \decisionproblem{SaturatedConfig} iff some saturated configuration of the TBN $\mathcal{T}$ has at least $k$ polymers.
\end{definition}

Most often we will be interested in configurations containing the maximum number of polymers (i.e. \textit{stable} configurations).

The software StableGen attempts to algorithmically determine the stable configuration(s) of a TBN and also allows the user to specify additional constraints that the configuration must satisfy (i.e. must group two specific monomers into a polymer).  It does this by specifying constraints to a \SAT\ solver (specifically, the default solver of the \texttt{PySAT} library), which acts as a black box.  The solution that this software provides to the \SAT\ instance also contains enough information to reconstruct a unique configuration of the original TBN with the correct number of polymers.

\subsection{StableGen Variables}
The (Boolean) variables used in the \SAT\ formulation are as follows:

\begin{itemize}
    \item Pair($s$, $t$): true iff binding site $s$ is bound to site $t$
    \item Bind(\monomer{m}, \monomer{n}): true iff monomer \monomer{m} is in the same polymer\footnote{In this paper we adopt the convention that Bind($\cdot$, $\cdot$) is reflexive, i.e. that Bind(\monomer{m}, \monomer{m}) is true for all monomers \monomer{m}.} as monomer \monomer{n}
    \item Rep(\monomer{m}): true iff monomer \monomer{m} is the representative (i.e. leader) monomer in its polymer, used to assist in counting the number of polymers
    % \item Sum($i$, $j$): true iff there are at least $j$ representatives amongst monomers
    % $\monomer{m}_1$, $\dots$, $\monomer{m}_i$,
    % used to provide a sense of numeracy to the \SAT\ formulation
\end{itemize}

I have omitted the description of the variables Sum($i$, $j$), which are used to provide a sense of numeracy in the formulation (specifically, for counting polymers).  These variables will be obviated by advances in the software tools used, allowing for (among other things) the specification of bounded linear inequalities.

\subsection{StableGen Constraints}

Note that $C(s)$ denotes the set of binding sites that are complementary to site $s$ and $L)$ denotes the set of limiting sites in the TBN.  We assume that there exists (i.e. the software assigns) an arbitrary ordering of the monomers.
\begin{align}
    \sum_{t \in C(s)}\text{Pair}(s,t) &\leq 1 &\forall s &\qquad  \text{no site is bound more than once}\label{stablegen-single-bonded}\\
    \sum_{t \in C(s)}\text{Pair}(s,t) &\geq 1 &\forall s \in L &\qquad  \text{all limiting sites are bound}\label{stablegen-saturation}
\end{align}

Note that constraint (\ref{stablegen-saturation}) ensures saturation of the configuration, since a configuration is saturated iff all limiting sites are bound.
\begin{align}
    \text{Pair}(s,t) \implies \text{Bind}(\monomer{m}, \monomer{n})
    & \qquad \forall \monomer{m}, \monomer{n} , \forall s \in \monomer{m}, \forall t \in \monomer{n}
    \label{stablegen-binding}\\
    \text{Bind}(\monomer{m}, \monomer{n}) \land \text{Bind}(\monomer{m}, \monomer{r}) \implies
    \text{Bind}(\monomer{n}, \monomer{r})
    & \qquad \forall \monomer{m}, \monomer{n}, \monomer{r}
    \label{stablegen-binding-transitivity}
\end{align}

Here constraint (\ref{stablegen-binding}) enforces that if two sites are paired, then their containing monomers must be in the same polymer, and (\ref{stablegen-binding-transitivity}) enforces the transitivity of this containment.  Note that in this model, two monomers may be in the same polymer even if they are not bound by any complementary sites.
\begin{align}
    \text{Bind}(\monomer{m}, \monomer{n}) \implies \lnot \text{Rep}(\monomer{n})
    & \qquad \forall \monomer{m} < \monomer{n} \label{stablegen-rep-ordering}\\
    \sum_\monomer{m} \text{Rep}(\monomer{m}) \geq k \label{stablegen-counting}
\end{align}

Here constraint (\ref{stablegen-rep-ordering}) ensures that there cannot be two representative monomers in the same polymer, and constraint (\ref{stablegen-counting}) enforces that the number of representatives must meet or exceed $k$.  Together, these constraints guarantee that the number of polymers in the configuration must meet or exceed $k$.  Note that this does not guarantee that each polymer will have a representative, but if a polymer with no representative was described in the solution, it would still satisfy constraint (\ref{stablegen-counting}), since for a set of polymers $P$, we have
\begin{equation*}
\abs{P}
= \sum_P 1
\geq \sum_P \sum_{\monomer{m} \in P} \text{Rep}(\monomer{m})
= \sum_\monomer{m} \text{Rep}(\monomer{m})
\geq k
\end{equation*}

\section{Solutions to Problem Scaling}

The efficiency of the solver acting upon the \SAT\ encoding depends greatly upon the amount of potential symmetry in the TBN.  Because the StableGen encoding considers every possible value for the Pair($\cdot$,$\cdot$) variables, it will consider (and report) all isomorphic configurations; that is, configurations which do not differ in their polymer composition, but in the manner in which those polymers are internally bound.  For instance, for $\mathcal{T} = \{\{a,a\}, \{a, a\}, \{a^*, a^*, a^*\}\}$, the solver will report 24 different configurations in which these three monomers are all grouped into a single polymer.
Given TBNs of sufficient complexity, StableGen can be quite slow as the solver must consider all isomorphic configurations in its search, even if one is able to remove redundancy via postprocessing.
Ideally, we would like to specify TBNs with a large amount of symmetry, either by including monomers that contain many binding sites of the same type, having a large number of equivalent configurations due to some underlying structure, or by specifying a large (possibly infinite) number of identical monomers.

For these reasons, it makes sense to consider an implementation that removes this sense of binding site pairing and replaces it with an equivalent notion that also guarantees saturation of the produced configuration.  We call such implementations \textit{bond-oblivious}.

\subsection{Constraint and Integer Programming}

\todoi{DH: Describe Constraint Programming and Integer Programming here, along with some description of the or-tools library.}

As IP solvers work by considering the convex relaxations of their related optimization problems, it is no longer sufficient to implement (\ref{stablegen-binding}), (\ref{stablegen-binding-transitivity}), and (\ref{stablegen-rep-ordering}) by implication (as an implication is a type of disjunction, and disjunctive statements about convex polyhedra are not convex).  That said, disjunctions of boolean variables are a much simpler affair, since if 1 represents true and 0 represents false, then $a \implies b$ can be implemented as $a \leq b$, and $a \land b \implies c$ can be implemented as $a + b \leq 1 + c$.  As such, the aforementioned constraints can be implemented as:

\begin{align}
    \text{Pair}(s,t) \leq \text{Bind}(\monomer{m}, \monomer{n})
    & \qquad \forall \monomer{m}, \monomer{n} , \forall s \in \monomer{m}, \forall t \in \monomer{n}
    \\
    \text{Bind}(\monomer{m}, \monomer{n}) + \text{Bind}(\monomer{m}, \monomer{r}) \leq
    1 + \text{Bind}(\monomer{n}, \monomer{r})
    & \qquad \forall \monomer{m}, \monomer{n}, \monomer{r}\\
    \text{Bind}(\monomer{m}, \monomer{n}) \leq 1 - \text{Rep}(\monomer{n})
    & \qquad \forall \monomer{m} < \monomer{n}
\end{align}

Additionally, both the CP and IP solvers admit an objective function, which in our case we will choose to be that $k$ is maximized in the solution configuration(s).  That said, the manner that the solvers approach this objective function is different, and while the CP solver can readily supply the enumerated set of solutions that reach the maximal value of $k$, the existing IP solvers do not natively provide the functionality to request the complete set of co-optimal solutions.

\todoi{
  DH: CP allows us to specify bounded linear inequalities which are algorithmically reduced to SAT variables, removing some reduction effort.  IP provides an alternate method which proceeds towards the optimal objective function differently, which in theory provides more efficient solutions because it does not require one to query the problem over and over for different values of $k$; however, the performance of IP is dubious when attempting to encode disjunctions, because an upper bound on the variables involved is required, and the larger this upper bound, the worse the condition number of the matrix provided to the numerical portion of the IP solver.  This restriction does not greatly affect the performance of IP on disjunctions of Boolean variables since each has an upper bound of 1.
}

\subsection{A Bond-Oblivious Implementation}

The most direct notion of a bond-oblivious model would simply remove all instances of Pair($\cdot$, $\cdot$) variables from the \SAT\ formulation, instead relying on the assignment of the Bind($\cdot$, $\cdot$) variables to describe a configuration.  Indeed, in addition to the benefit of having fewer variables, constraints (\ref{stablegen-single-bonded}), (\ref{stablegen-saturation}), and (\ref{stablegen-binding}) would also seem unnecessary.  However, these constraints contained one important piece of information which would now be unenforced: the configuration specified by the solution must be saturated.

If it is not permitted to specify the exact matching between the binding sites, how else is it possible to enforce that the limiting sites are bound?  To solve this problem, the formulation must include some concept of numeracy.  Specifically, it must be able to tally the site content of each polymer, checking each to ensure that any excess limiting sites are not exposed; a configuration is saturated if and only if each polymer in the configuration has no exposed limiting sites \cite{ktbn}.

The added flexibility of CP and IP solvers allow us to embed this sense of numeracy directly into the encoding.  Let $\monomer{n}(t)$ denote the ``net count of $t$ in \monomer{n}'': the difference between the count of sites of type $t$ in \monomer{n} and the count of the sites of complementary type $C(t)$ in \monomer{n}.  Let $L'$ denote the set of limiting binding site types.  As the solvers consider Boolean variables to be 1 (true) or 0 (false), and allows linear inequalities, we can now encode this constraint in the following manner:

\begin{align}
    \sum_\monomer{n}\text{Bind}(\monomer{m}, \monomer{n})\cdot \monomer{n}(t) \geq 0
    & \qquad \forall \monomer{m}, \forall t \not\in L'
\end{align}

Specifically, for each polymer we must guarantee that the number of limiting sites its monomers has is fewer than the number of corresponding complementary sites (equivalently, the net count of sites that are not limiting must be non-negative).  The intention is to enforce this for each polymer, guaranteeing saturation; however, as the formulation has no direct notion of polymer, we instead enforce this by prescribing that for all monomers, the polymer that contains the monomer must obey the constraint.  Since each polymer contains at least one of the monomers, the limiting site constraint is satisfied for all polymers.

\subsection{A Multiset Implementation}\label{multiset-implementation}

\todom{DH: Said differently, there are no longer any ``labelled monomers''}

A seemingly natural extension to the formulation of the previous section would be to add the ability to specify the TBN as a multiset of monomers, rather than specifying each monomer individually.  Recalling that we would like to be able to specify a large number of copies of a monomer, needing to specify each monomer individually in the TBN not only increases the input size of the problem, but also contributes factorially to the symmetry of the solution set.  For instance, if five of the same monomer type are specified, for each true solution it will produce as many as $5!$ times as many solutions in which the identical monomers have been permuted in various ways.

A difficulty in extending the formulation to allow for such multisets arises from how the polymers are specified.  If, as before, they are specified with pairwise Bind($\cdot$, $\cdot$) variables, solution symmetries will persist (in very similar fashion to why the Pair($\cdot$, $\cdot$) variables were removed previously).  One could also choose to specify Bind($\cdot$, $\cdot$) variables to be nonnegative integer variables rather than Boolean variables, but then the transitive constraints would not work; if Bind($\monomer{m}_1$, $\monomer{m}_2$) $= 1$ and Bind($\monomer{m}_2$, $\monomer{m}_3$) $= 1$, it is not clear if this should imply that Bind($\monomer{m}_1$, $\monomer{m}_3$) $\geq 1$, since it could be the case that the earlier bindings were affected by different instances of $\monomer{m}_2$.

\todoi{DH: this is a good place to loop in theory about combinatorial auctions, to which this problem is very closely related}

A more promising direction then is to specify the polymers not by inferring their composition from the binding relationships of the monomers, but instead to include in the formulation an explicit list of monomer counts in each polymer.  It is not possible to know \textit{a priori} how many such polymers will be formed, but a simple upper bound presents itself: the number of polymers cannot exceed the number of monomers in the system.  Additionally, if solving the decision problem \decisionproblem{SaturatedConfig}, then the number of polymers $k$ is already given as input to the problem.\todom{DH: If cannot make $k$ ``clean'' polymers but can make more than $k$ clean polymers, this will still be acknowledged by solutions that include spurious binding to reduce the number of polymers back to $k$... although the available choices of which polymers to spuriously bind will greatly enlarge the solution set.}

\todoi{DH: An explanation of why it is generally intractable to generate the full set of ``possible polynomials`` a.k.a. ``packing schemes'' would be useful here -- as the full set could be exponentially large, requires accounting for additional ``slack'' monomers, and requires the generation of a Graver basis set.\\\ \\
That said, this approach is not without merit, and could be useful if we have \textit{a priori} knowledge that the basis set will be reasonably sized (for instance, because our construction is fairly rigid, as in the classic grid gate).  In this case, the algorithm would work in two stages: (1) Generate the first-orthant elements of a Graver basis, (2) Determine nonnegative coefficients for the basis vectors.\\\ \\
Said differently, these tasks would be: (1) Determine the different types of locally saturated polymers that are possible to build, and (2) determine how many of each polymer type should be built in order to exhaust either the monomer supply or the limiting site supply.}

To specify this in the formulation, Stable-TBN uses the following variables:

\begin{itemize}
    \item Count(\monomer{m}, $j$): the integer count of monomers of type $\monomer{m}$ contained in polymer $\polymer{P}_j$
    \item Nonempty($j$): false if polymer $\polymer{P}_j$ is empty, possibly true otherwise
\end{itemize}

The observant reader may notice that the variable $Nonempty(\cdot)$ is not guaranteed to be true in the case that a polymer is nonempty; however, as the purpose of this variable is ultimately to count the number of nonempty polymers, any false negative will only serve to undercount the number of polymers and so will not restrict the solution set.

Assume an arbitrary ordering of the monomer types.  Let $\#(\monomer{m})$ denote the number of monomers of type \monomer{m} in the TBN.  Let B be an upper bound on the number of polymers.  The constraints that encode the proper meaning of the variables are as follows:

\begin{align}
    \sum_{j=1}^B\text{Count}(\monomer{m},j) &= \#(\monomer{m})
     &\forall \monomer{m} \in \mathcal{T}
     &\qquad \text{all monomers must be in a polymer}\label{stabletbn-inclusion}\\
    \sum_\monomer{m}\text{Count}(\monomer{m}, j)\cdot \monomer{m}(t) &\geq 0
     &\forall j \in [1..B], \forall t \not\in L'
     &\qquad \text{all limiting sites are bound}\label{stabletbn-limiting-domain}\\
    \sum_\monomer{m}\text{Count}(\monomer{m}, j) &\geq \text{Nonempty}(j)
     &\forall j \in [1..B]
     &\qquad \text{Polymer is empty if no monomers}\label{stable-tbn-nonempty}\\
    \sum_{j=1}^B\text{Nonempty}(j) &\geq k
     &
     &\qquad \text{must have at least $k$ polymers}\label{stable-tbn-polymer-count}
\end{align}

Optionally, the solver can be instructed to maximize the value of $k$.

These constraints are sufficient to produce correct answers from the solver, but they do not remove all symmetric answers for the following reason: this encoding produces an ordering on the polymers (i.e. $\polymer{P}_1, \dots, \polymer{P}_B$), but there is no reason that the solver should restrict its solutions to a single ordering, instead producing \textit{all} possible orderings of the polymers.  We must then choose a target ordering to remove this symmetry, and while there are many choices for this ordering, for simplicity we choose the (descending) lexicographical ordering induced by the order of the monomer types.

If using an IP solver, which produces only one solution from the set, the ordering of the solution is not important to uniqueness, although it is possible that enforcing an ordering may reduce the size of the search space, resulting in faster runtime.  That said, it is not immediately clear if this benefit offsets the performance decline by encoding a sorting algorithm into the formulation\todom{DH: I've tried both and while there is a difference, it's not big, and it can go either way depending upon the specific input}, for sorting in an IP is already a difficult task (for instance, see \cite{ip-sorting}).  The primary reason for this difficulty is that encoding a sorting involves logical implications, which, being a type of disjunction, are difficult to encode into a convex formulation.  We do have an upper bound on the values that the Count($\cdot$, $\cdot$) variables can take, making certain ``large-number'' techniques possible; formulations including these techniques are discussed in the appendix.\todom{DH: make an appendix}

If using a CP solver, enforcing an ordering provides a signficant boost to efficiency precisely because it reduces the available search space (as well as the more obvious benefit of producing non-isomorphic solutions).  This is achieved by establishing a new set of variables for each consecutive pair of polymers $\polymer{P}_{j-1}$, $\polymer{P}_{j}$:

\begin{itemize}
    \item Tied($\monomer{m}_i$, $j$): true if Count($\monomer{m}_h$, $j-1$) 
     $=$ Count($\monomer{m}_h$, $j$) $\forall h \leq i$
\end{itemize}

As a base case, we establish the convention that Tied($\monomer{m}_0, j$) is true for all $j$.

Intuitively, when comparing two lists of scalars (i.e. vectors) to verify that they are correctly sorted, one must proceed down the list of entries until one of the entries is larger than its corresponding entry in the other list.  For as long as the numbers are the same, they are considered ``tied''.  When one entry exceeds the corresponding other, the tie is considered ``broken'', after which no further comparisons need be conducted between the two vectors.  The meaning of these variables is enforced by the following constraints:

\begin{align}
    \text{Tied}(\monomer{m}_i, j) &\implies \text{Tied}(\monomer{m}_{i-1}, j)
     &\qquad\forall i, \forall j \in [2..B]\label{stabletbn-tiebreak-grandfather}\\
    \text{Tied}(\monomer{m}_i, j) &\implies \qty\big(\text{Count}(\monomer{m}_i, j-1) =
     \text{Count}(\monomer{m}_i, j))
     &\qquad\forall i, \forall j \in [2..B]\label{stabletbn-tiebreak-equal}\\
    \lnot\text{Tied}(\monomer{m}_i, j) \land \text{Tied}(\monomer{m}_{i-1}, j)
     &\implies \qty\big(\text{Count}(\monomer{m}_i, j-1) >
     \text{Count}(\monomer{m}_i, j))
     &\qquad\forall i, \forall j \in [2..B]\label{stabletbn-tiebreak-broken}
\end{align}

Intuitively, (\ref{stabletbn-tiebreak-grandfather}) enforces that a tie is only relevant if it is not resolved by a previous entry, (\ref{stabletbn-tiebreak-equal}) enforces that ties can only continue if the entries are equal, and (\ref{stabletbn-tiebreak-broken}) enforces that ties can only be broken if the tie was not broken previously and the current entries are ordered correctly.

In this manner, any solution verifying the constraints must obey the induced ordering on the polymers.

\subsection{Unbounded Count Multisets}

While the multiset implementation of the previous section allows for the analysis of increasingly complex TBNs in an efficient manner, it still does not deliver on the intended use case of specifying ``excess'' monomers; that is, monomers present in an essentially infinite quantity (e.g. ``fuel species'').  Indeed, even for some mildly ambitious TBNs, the computation is delayed by the following: our typical use cases generally result in configurations with a large number of singleton polymers (i.e. polymers with only one monomer).  The added computational load of handling all these polymers explicitly is both inefficient and unnecessary.\todom{DH: So, for instance, handling 3x3 catalyzed grid gate with 2 Gs, 1C, and around 10 of each fuel is about the limit before performance substantially drops off -- these numbers are from memory, so I need to run this again to check the exact numbers.  It continues to run really well for most size grid gates when fuels are in quantity lower than 5.}

One observation is that in these desired use cases, the actual computational difficulty of the underlying problem is not in assigning all of the monomers to polymers, but instead on the assignment of monomers that contain limiting sites (we will refer to these as \textit{limiting monomers}).  Since a binding site on a monomer with infinite quantity cannot be a limiting site, we can restrict our focus to the subset of limiting monomers.  The question of maximizing the number of polymers in the configuration then becomes an equivalent question about the difference between how many monomers from outside the subset must be recruited to saturate the system and how many non-singleton polymers are created.  Intuitively, this expression gives the number of pairwise merge operations that must be performed in order to produce the final configuration if starting from the all-singletons configuration.\todom{DH: Intuition: for grid gate I only need to know how the Gs are bound up, and I can infer the rest.  Similarly, for a system dominated by top strands, I only need to know how the bottom strands are bound up.}

More formally, whereas we had previously maximized $k$ in order to describe configurations with a large number of polymers, we could have equivalently minimized $|\mathcal{T}| - k$ (minimizing the number of merges required to construct the configuration).  For finite values of $|\mathcal{T}|$ and $k$ this difference can be evaluated, but if excess monomers are allowed, both values could be infinite.  Instead, we can focus on the task of determining a partial configuration $\alpha$ containing all of the limiting monomers and the corresponding set of merged monomers $\bigcup_{\polymer{P} \in \alpha} \polymer{P}$ that minimize the number of merges necessary to create the partial configuration (and by extension, the full configuration that includes the singletons):

\begin{equation}
    \min_{\alpha} \qty(\qty(\sum_{\polymer{P} \in \alpha} |\polymer{P}|) - |\alpha|)
\end{equation}

Recall that the previous formulation requires an upper bound $B$ on the number of polymers formed, which could be specified by the user, equal to $k$ when solving the decision version of the problem, or conservatively chosen to be the number of monomers in the system.  In this case, we will want to similarly use an upper bound ($B'$) on the number of non-singleton polymers formed.  Again, this can be specified by the user, formulated as input to a decision problem, or conservatively taken to be the count of limiting monomers.

In this version, we retain the same variables as in the previous formulation: Count($\monomer{m}$, $j$), Nonempty($j$), and Tied($\monomer{m}_i$, $j$).  Note that in this new version $j$ will range over $[1..B']$ rather than $[1..B]$.  Let $\mathcal{T}_{L'}$ denote the set of limiting monomers.

The constraints can be modified to our new purpose as follows:

\begin{align}
    \sum_{j=1}^{B'}\text{Count}(\monomer{m},j) &= \#(\monomer{m})
     &\forall \monomer{m} \in \mathcal{T}_{L'}
     &\qquad \text{all limiting monomers must be in a polymer}\label{stabletbn-inf-strict-inclusion}\\
    \sum_{j=1}^{B'}\text{Count}(\monomer{m},j) &\leq \#(\monomer{m})
     &\forall \monomer{m} \in \mathcal{T}\setminus\mathcal{T}_{L'}
     &\qquad \text{cannot exceed monomer supply}\label{stabletbn-inf-bounded-inclusion}\\
    \sum_{\monomer{m} \in \mathcal{T}}\text{Count}(\monomer{m}, j)\cdot \monomer{m}(t) &\geq 0
     &\forall j \in [1..B'], \forall t \not\in L'
     &\qquad \text{all limiting sites are bound}\label{stabletbn-inf-limiting-domain}\\
    \sum_{\monomer{m} \in \mathcal{T}_{L'}}\text{Count}(\monomer{m}, j) &\geq \text{Nonempty}(j)
     &\forall j \in [1..B']
     &\qquad \text{Polymer is empty if no limiting monomers}\label{stable-inf-tbn-nonempty}\\
    \sum_{j=1}^{B'}\text{Nonempty}(j) &\geq k
     &
     &\qquad \text{must have at least $k$ polymers}\label{stable-inf-tbn-polymer-count}
\end{align}

The tiebreaking constraints (\ref{stabletbn-tiebreak-grandfather}), (\ref{stabletbn-tiebreak-equal}), and (\ref{stabletbn-tiebreak-broken}) are also taken verbatim with the exception that $B$ is replaced by $B'$.

\todoi{DH: Distinguish between ``limiting'' and ``limited'' monomers while making clear the meaning and use of constraints (19) and (20)}

\todoi{DH: Need some benchmarking of the new formulation.}

\subsection{Low-W formulation}

\todoi{DH: This is implemented. Needs formulation and documentation.}
